# Supplementary material for: The Symmetry Basis of Pattern Formation in Reaction-Diffusion Networks
Source: arXiv:2101.10434 source file (2021-02-26)

(a) Stability of Kuramoto network  
invariant manifolds

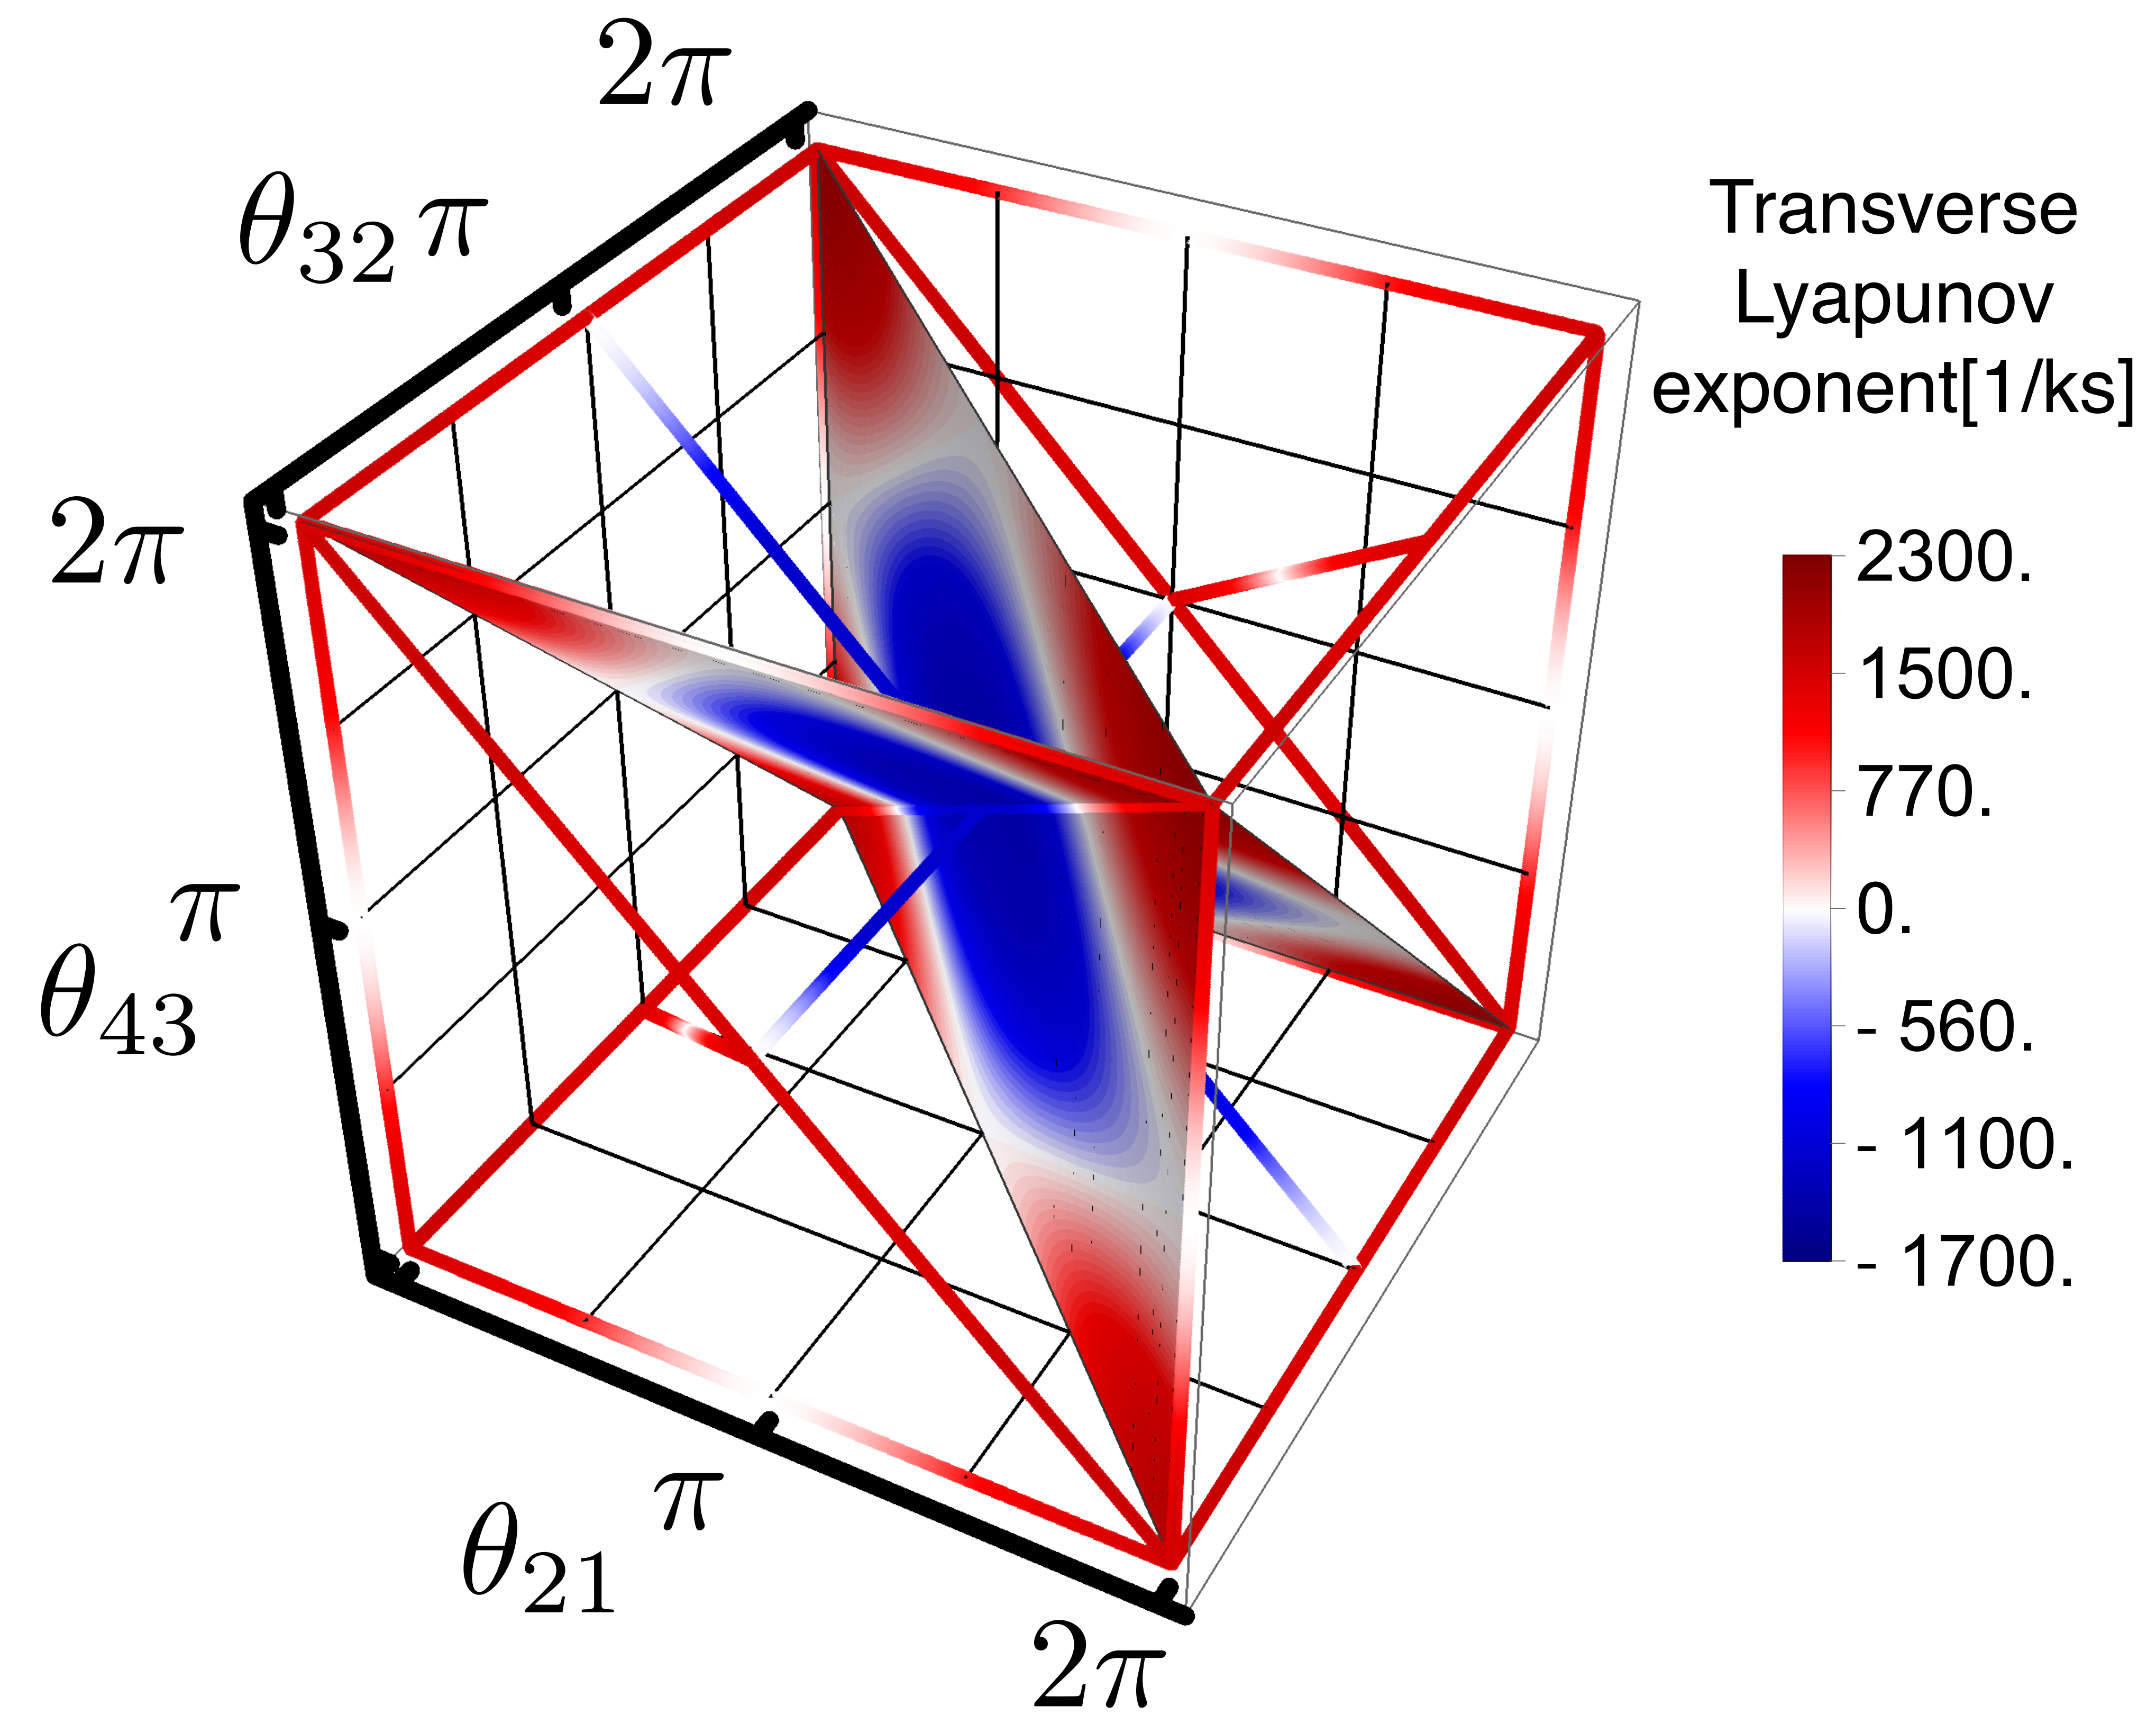

(b) Stability of BZ network  
invariant manifolds

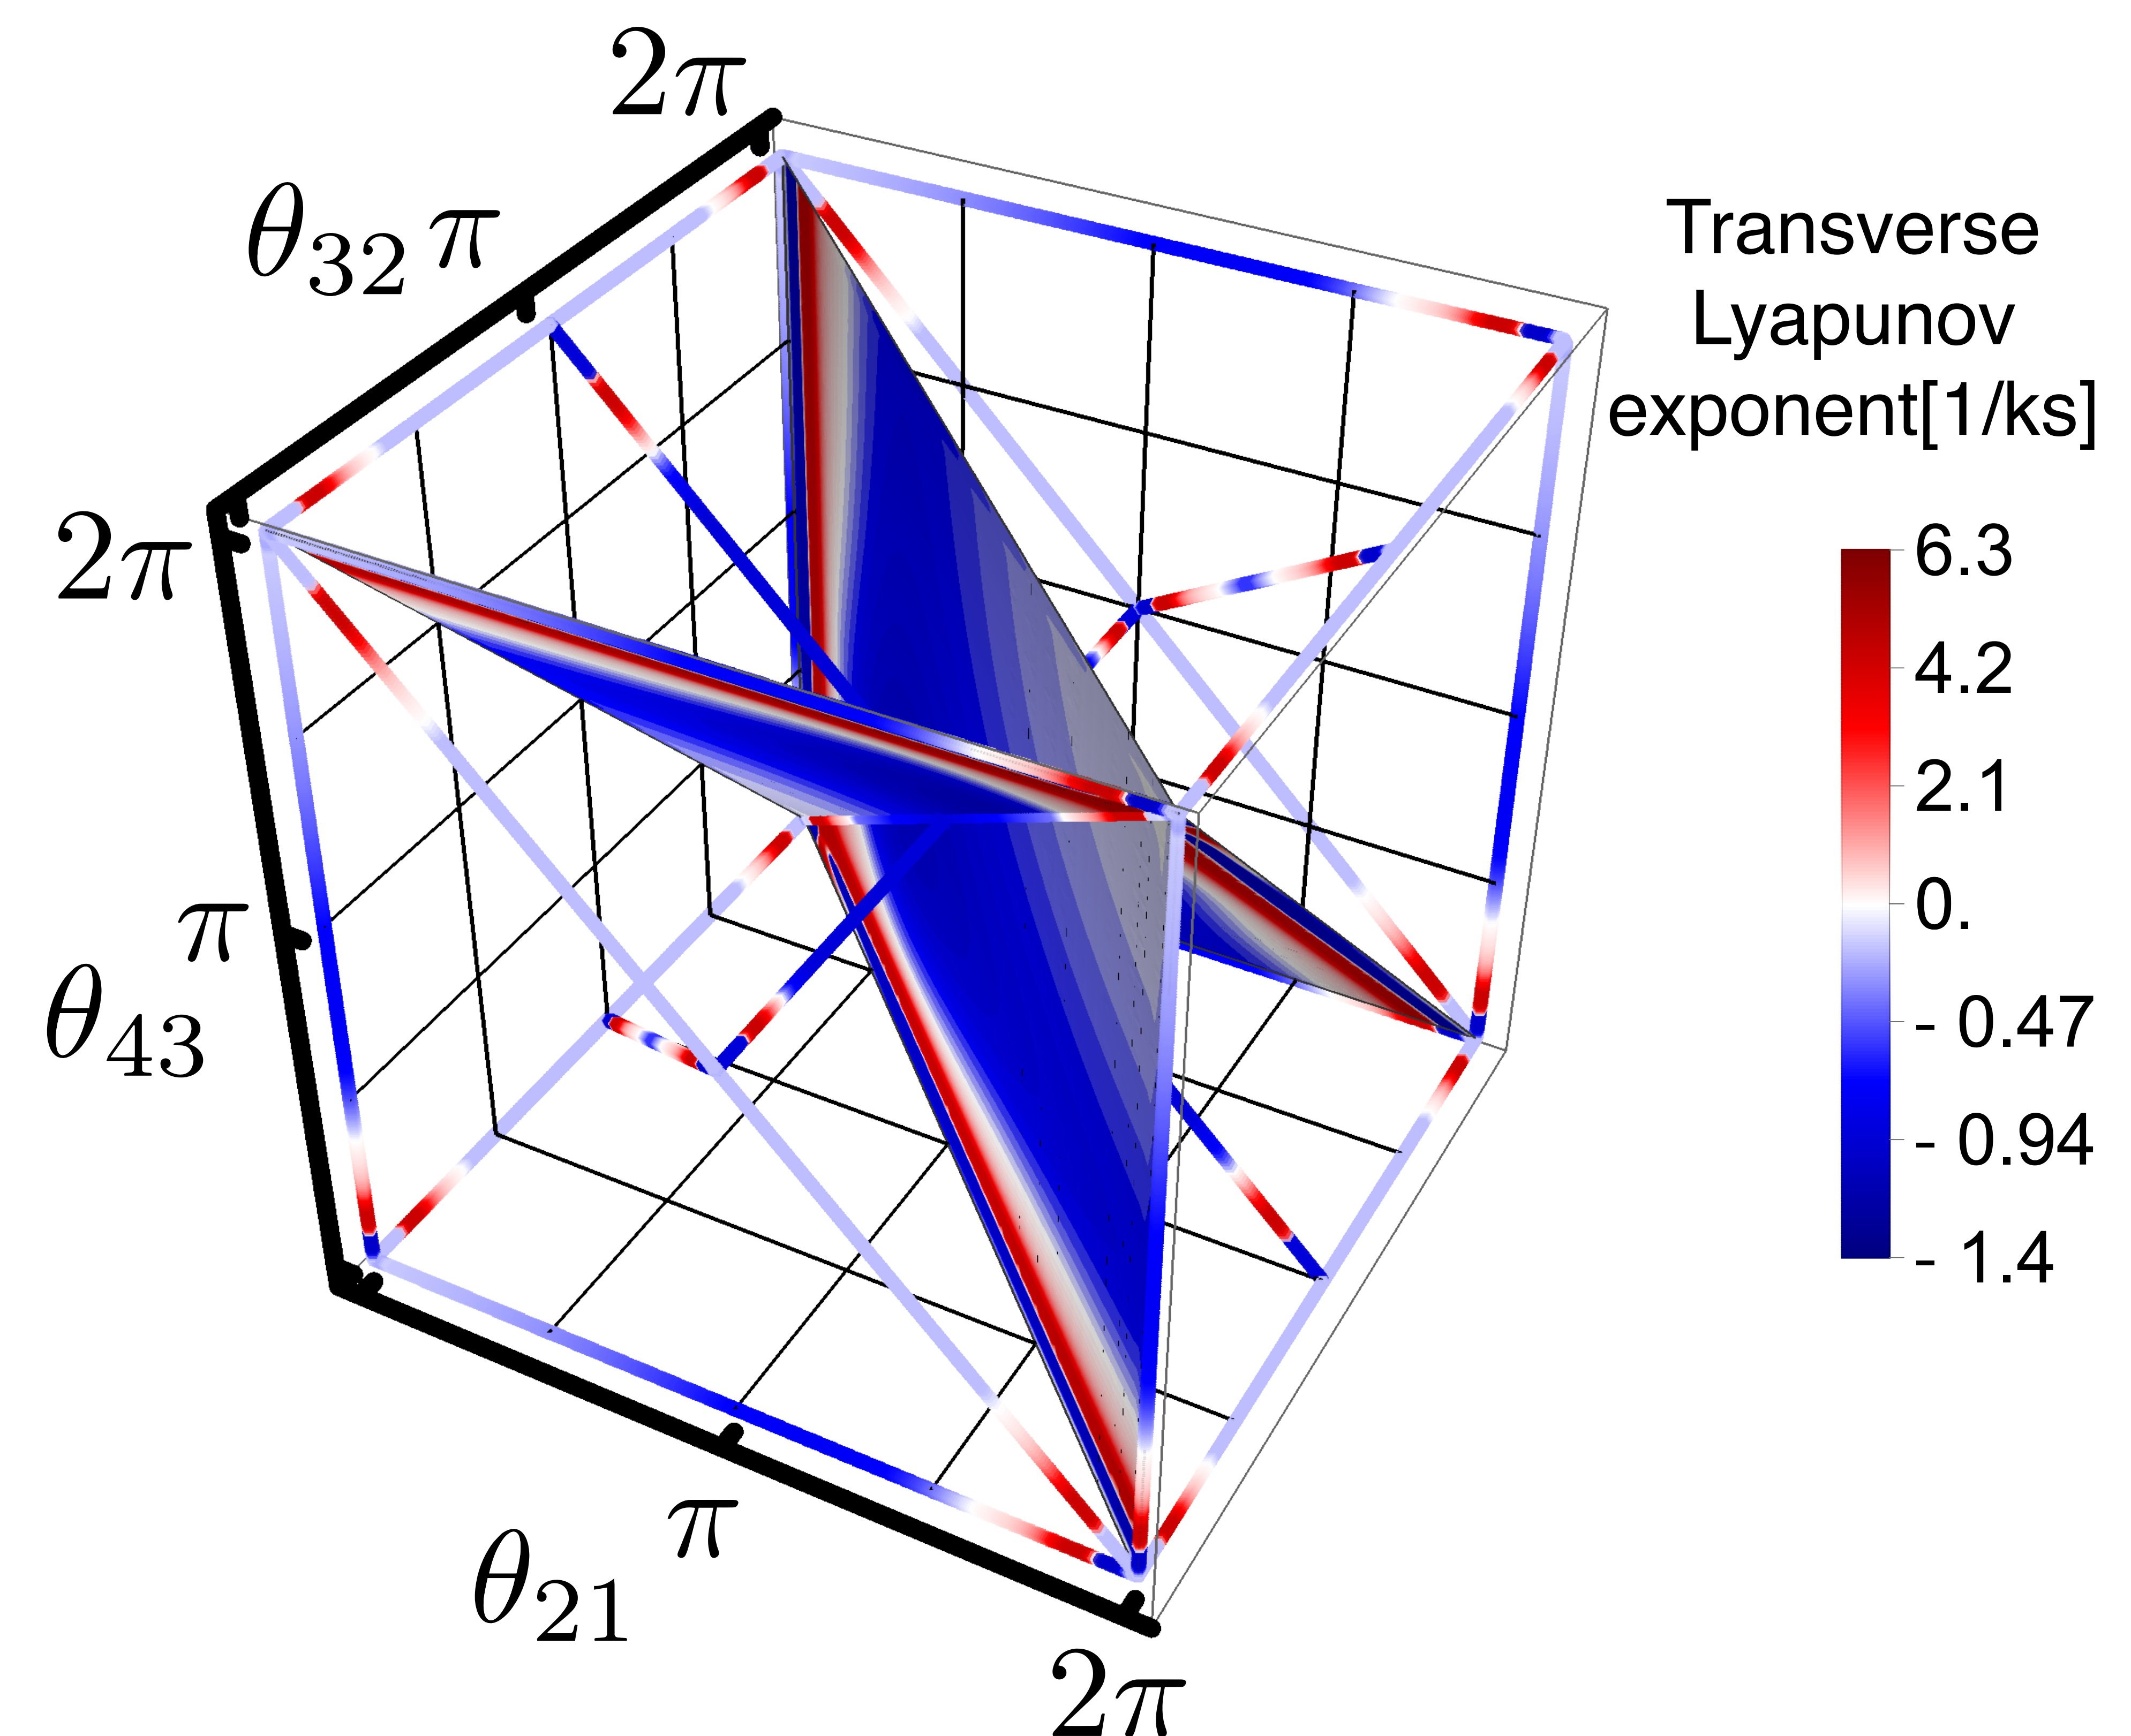



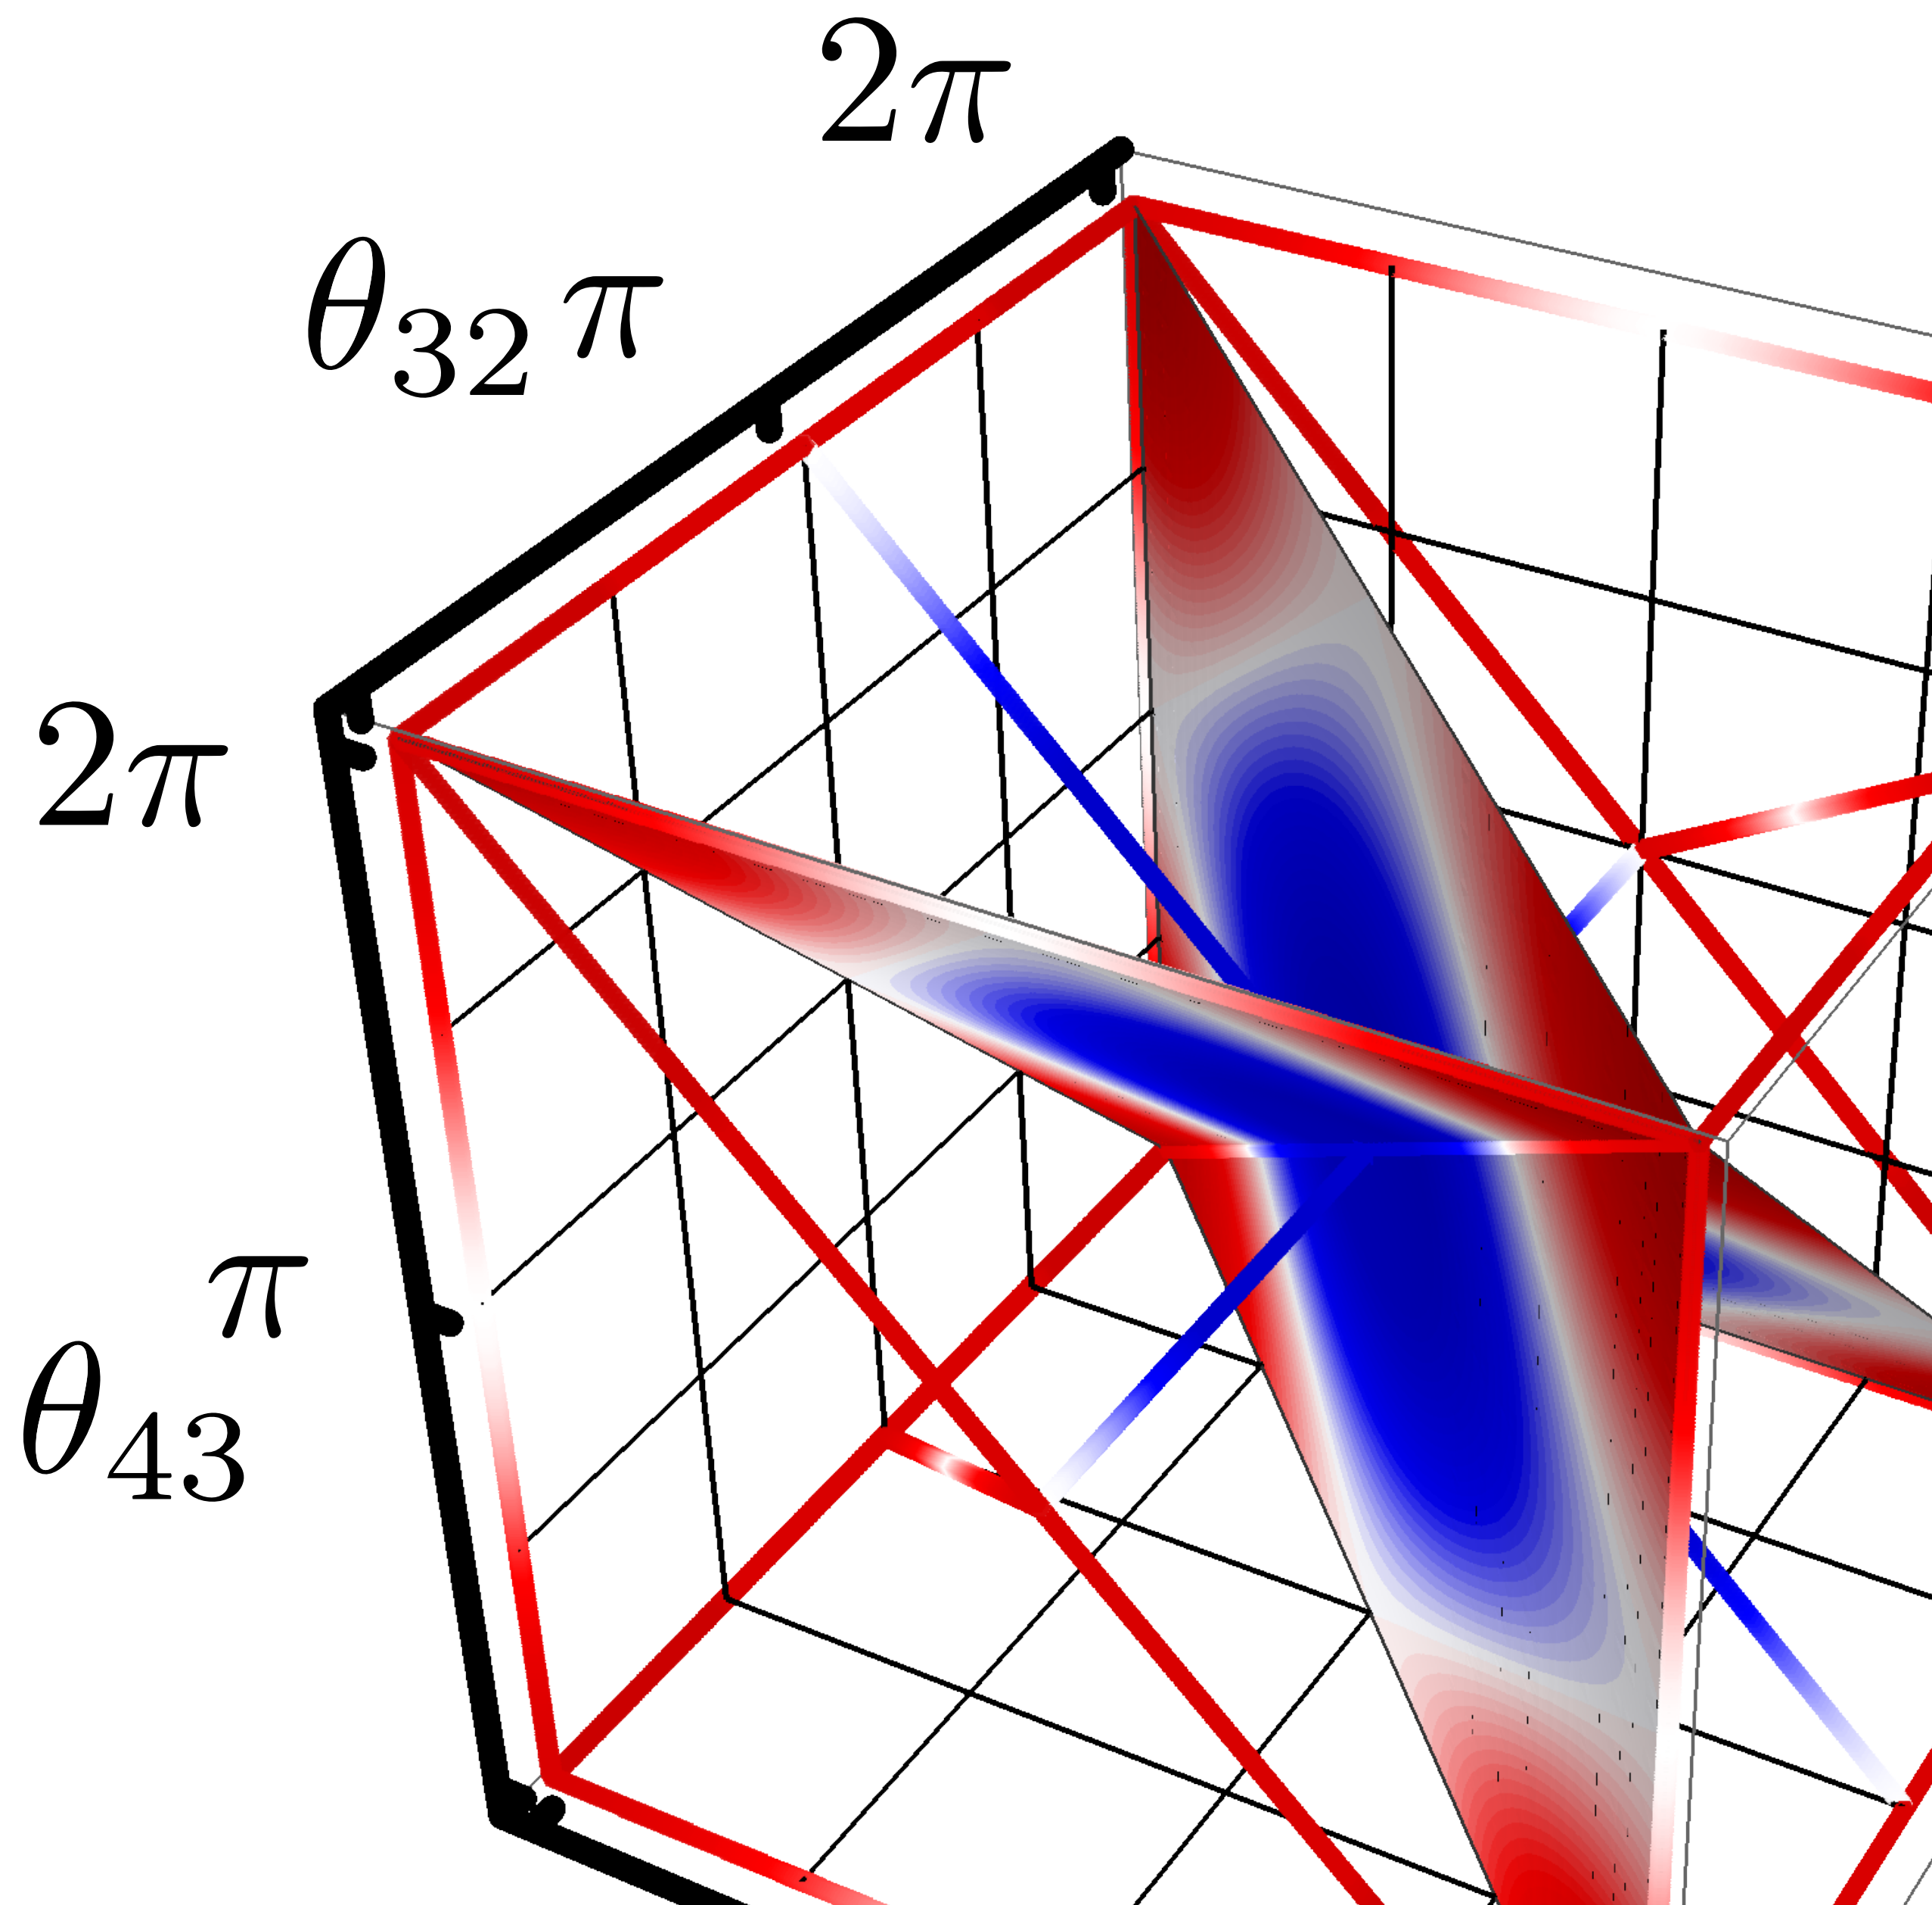

Supplement: Supplementary file 2 [file CombinedKuraAndBestFit.pdf]
